# Supplementary material for: Informing policy via dynamic models: Cholera in Haiti
Source: arXiv:2301.08979 source file (2024-03-04)
Supplement: Supplementary file 2 [file si_files_template.tex]

\documentclass[11pt]{article}

\input{inputs/header}

\usepackage{titlesec}
\usepackage{chngcntr}
\usepackage{etoolbox}

% Remove the numbering from sections
\titleformat{\section}{\normalfont\Large\bfseries}{}{0pt}{}

% Reset the subsection counter at the start of each section
\counterwithin*{subsection}{section}

% Change the numbering for subsections to have an S prefix and remove chapter numbering
\renewcommand{\thesubsection}{S\arabic{subsection}}

% Increment the subsection counter every time a subsection is created
% \pretocmd{\subsection}{\stepcounter{subsection}}{}{}

\usepackage[labelformat=empty]{caption}

\begin{document}

%%%%%%%%%% START

%%%%%%%%%% END

\clearpage

\bibliography{../bib-haiti}

\end{document}
